# Supplementary material for: Strain-Driven Thermal and Optical Instability in Silver/Amorphous-Silicon Hyperbolic Metamaterials
Source: arXiv:2207.09571 ancillary file (2022-07-19)
Supplement: Supplementary file 1 [file supplementary.pdf]

Supporting Information for  
**Strain-Driven Thermal and Optical Instability in  
Silver/Amorphous-Silicon Hyperbolic  
Metamaterials**

Jose L. Ocana-Pujol<sup>1,\*</sup>, Lea Forster<sup>1,2</sup>, Ralph Spolenak<sup>1</sup>, and Henning  
Galinski<sup>1,\*</sup>

<sup>1</sup>Laboratory for Nanometallurgy, Department of Materials, ETH Zurich,  
Zürich, Switzerland

<sup>2</sup>Laboratory of Multifunctional Ferroic Materials, Department of Materials,  
ETH Zurich, Zürich, Switzerland

\*corresponding authors, E-mail: joseo@ethz.ch and  
henningg@ethz.ch

# 1 Optical properties of the sputtered films

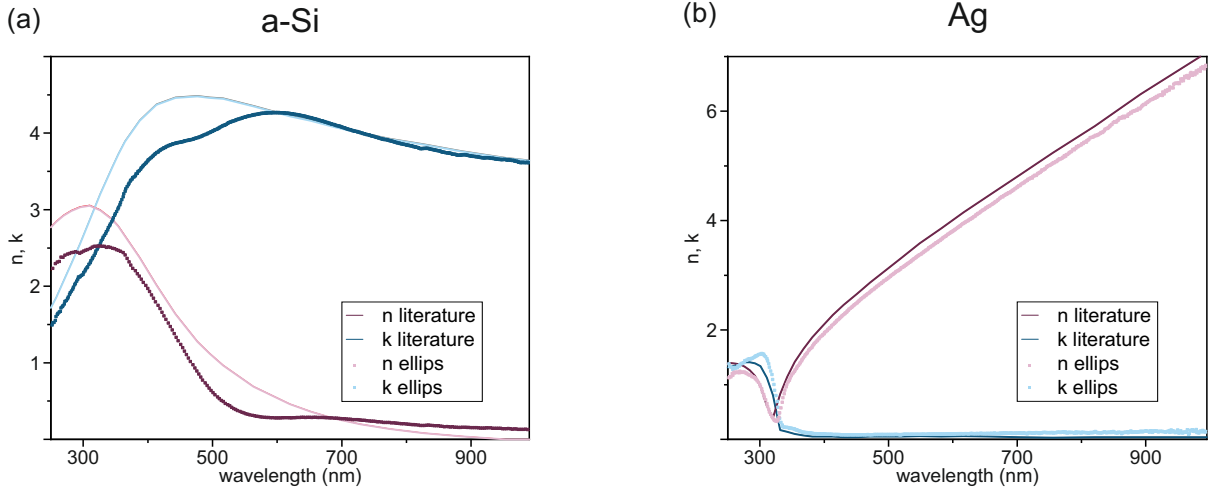

Figure S1: Comparison of the complex refractive index (n, k) measured by ellipsometry with values from literature for (a) Ag [1] and (b) a-Si[2].

## 2 Transfer Matrix Calculations

In order to better understand the physics behind the transitions in the measured reflectance ratio  $R_p/R_s$  in the main text (see Figure 1) , the reflectance at different angles and polarization was calculated using the Transfer Matrix method [3]. The calculated  $R_p/R_s$ ,  $R_p$  and  $R_s$  color maps together with the experimental results are shown in **Figure S2**. For all the considered Ag contents, a significant drop in the reflectance at s-polarization is expected at the transition wavelengths between a Brewster-angle-supporting topology (HMM type 1 or dielectric) and an SPP-supporting topology (HMM type 2 or metallic), resulting in an inversion of the  $R_p/R_s$  ratio. This drop is only moderate in our measured values.



This indicates that the match between the effective medium approximation and the experimental results cannot be fully understood by considering perfectly flat layers. Introducing a mean roughness in the system closes the gap between the calculated and measured reflectance. To account for roughness, the Modified Transfer Matrix method was used [4][5]. In this method, the reflectance and transmittance coefficients are modified as follows:

$$r_{ij,MTM} = r_{ij,TM} * e^{-\frac{4\pi\sigma^2}{\lambda} n_i^2}, \quad (1)$$

$$t_{ij,MTM} = t_{ij,TM} * e^{-\frac{4\pi\sigma^2}{\lambda} (n_i - n_j)^2}. \quad (2)$$

Where  $\sigma$  is the roughness and the  $i$  and  $j$  subscripts refer to the different layers. The roughness was fitted using the reflectance at normal incidence. It was found that in order to obtain a fit with a sufficient  $R^2$ ,  $\sigma$  needed to be heterogeneous, meaning that  $\sigma_{ij} > \sigma_{ji}$ . **Figure S3** shows the  $R^2$  coefficients for a variety of  $\sigma_{Ag,Si}$  and  $\sigma_{Si,Ag}$  and illustrates the need for the asymmetry in roughness with some examples of two different multilayers with different bilayer thicknesses and Ag content. The limit of roughness ensuring continuity of the film is given by:

$$\sigma_{Ag,Si} = \frac{\frac{h_{Ag}}{h_{bilayer}} - \sigma_{Si,Ag}}{\sqrt{2}}. \quad (3)$$

The normal reflectance spectra in Figure S3 are the fits with the highest  $R^2$  with an 80% of the maximum roughness as defined in equation 3 and have either symmetrical roughnesses or a 5:1  $\sigma_{Si,Ag}/\sigma_{Ag,Si}$  ratio. The fact that the roughness above Ag layers is larger can be explained by the higher power used to deposit Ag (DC 300W) compared with the values for Si deposition. This effect has been studied in literature [6]. Therefore, heterogeneity in the roughness underlines the importance of taking into account the specific deposition conditions when studying the optical properties of these multilayers.

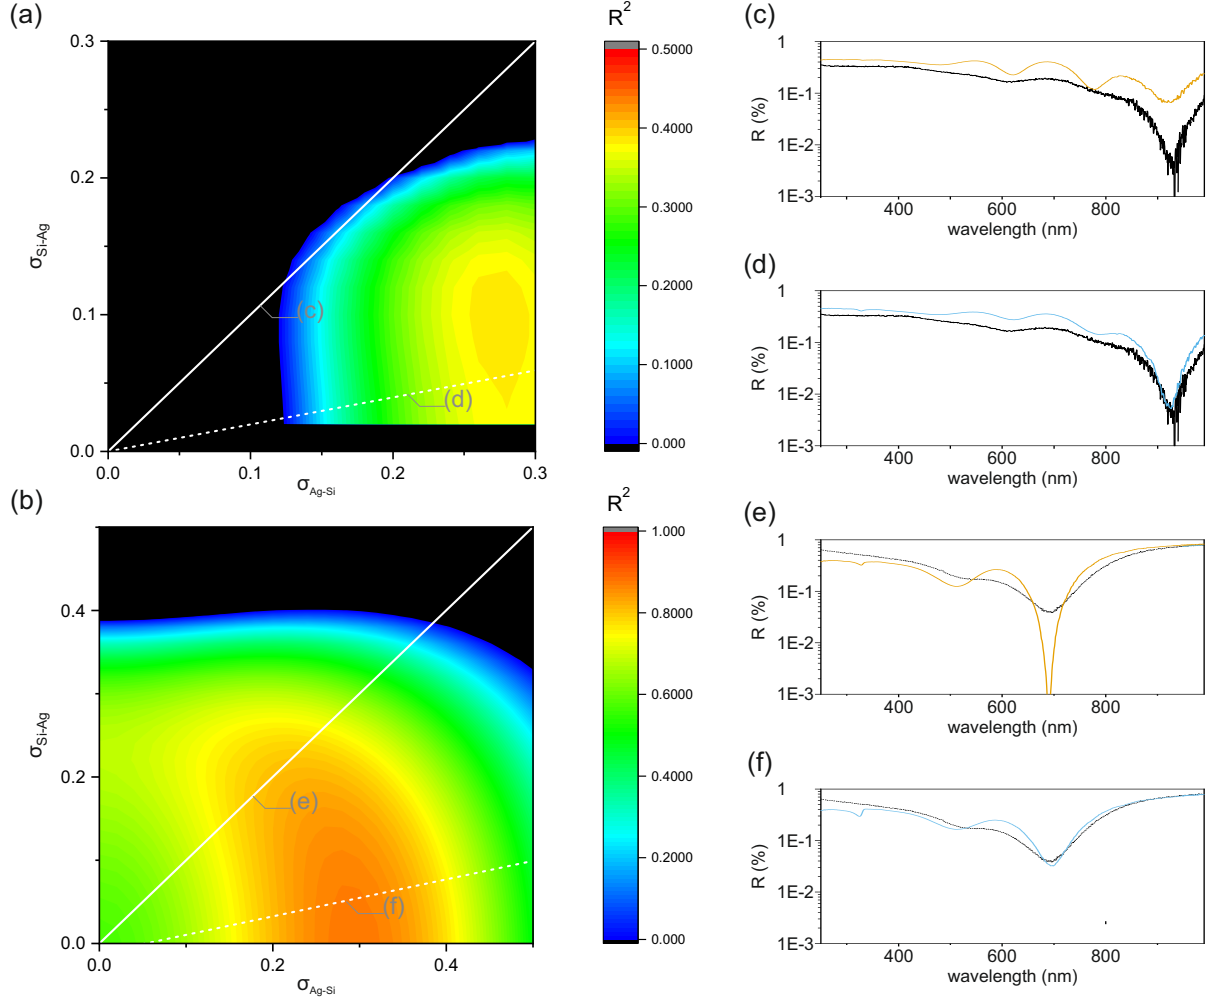

Figure S3: (a) and (b):  $R^2$  coefficients obtained by fitting the reflectance at normal incidence of the 30 vol.% Ag, 40 nm bilayer thickness (a) and the 50 vol.% Ag, 30 nm bilayer thickness design (b) against MTM calculated reflectances for different roughness values. The white lines indicate  $\sigma_{\text{Ag,Si}} = \sigma_{\text{Si,Ag}}$  (solid) and  $\sigma_{\text{Ag,Si}} = 5\sigma_{\text{Si,Ag}}$  (dashed). (c) and (d): Comparison between the measured and simulated reflectance at normal incidence of the 30 vol.% Ag, 40 nm bilayer thickness system when the roughness parameters are  $\sigma_{\text{Ag,Si}} = \sigma_{\text{Si,Ag}} = 0.108$  (c) and  $\sigma_{\text{Ag,Si}} = 0.044$  and  $\sigma_{\text{Si,Ag}} = 0.22$ . (e) and (f): Comparison between the measured and simulated reflectance at normal incidence of the 50 vol.% Ag, 30 nm bilayer thickness system when the roughness parameters are  $\sigma_{\text{Ag,Si}} = \sigma_{\text{Si,Ag}} = 0.18$  (e) and  $\sigma_{\text{Ag,Si}} = 0.057$  and  $\sigma_{\text{Si,Ag}} = 0.287$ .

**Figure S4** shows how the calculated the  $R_p/R_s$ ,  $R_p$  and  $R_s$  color maps compare to the measured values with and without introducing roughness. The introduction of asymmetrical roughness results in a more moderate drop of the reflectivity with s-polarized light and in a broadening in the p-polarized case, which is in good agreement with the measured  $R_p/R_s$  ratio.

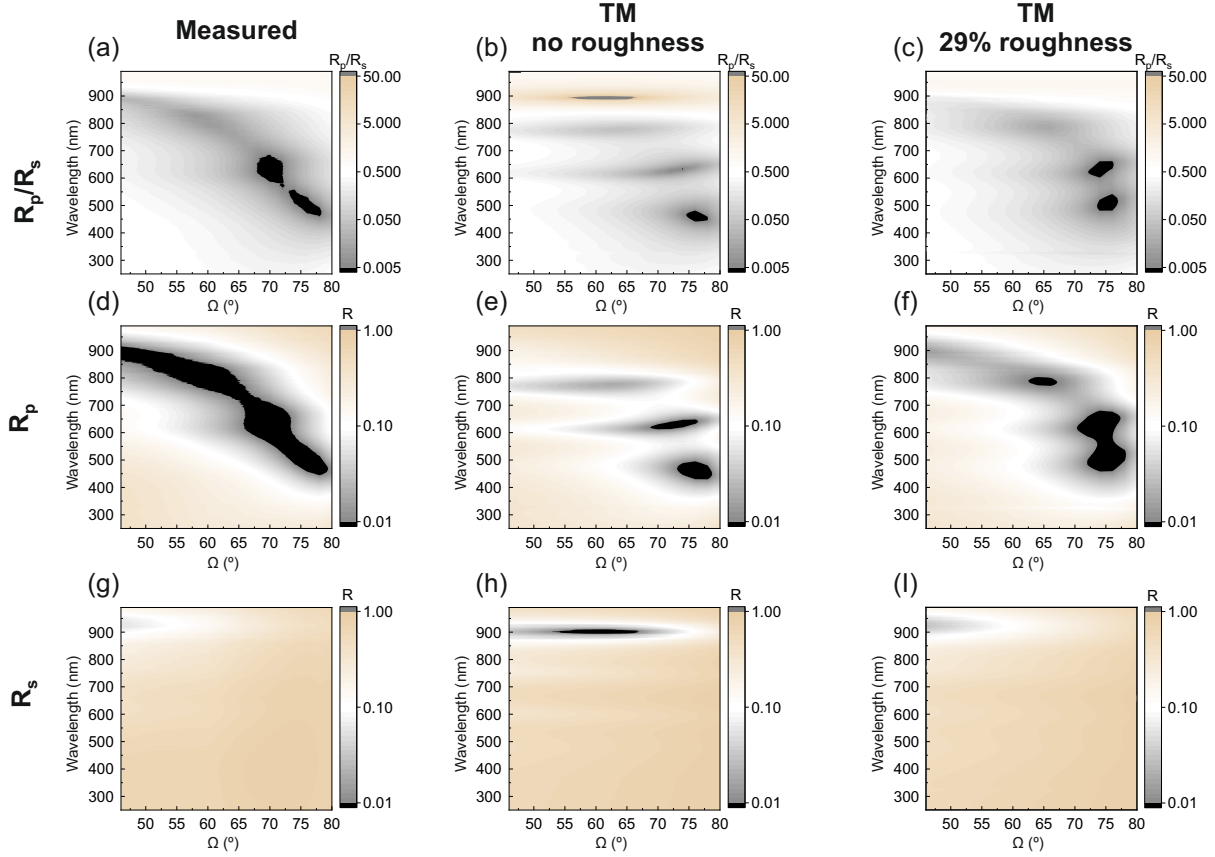

Figure S4: Comparison between the experimental and calculated optical properties of the system with 30 vol.% Ag content for a bilayer thickness of 40 nm. (a), (b) and (c): Ratio between the reflectance of p- and s-polarized light (a) measured experimentally, (b) calculated without roughness and (c) calculated with a 41% roughness. (d), (e) and (f): Reflectance at p-polarization (d) measured experimentally, (e) calculated without roughness and (f) calculated with a 41% roughness. (g), (h) and (i): Reflectance at p-polarization (g) measured experimentally, (h) calculated without roughness and (i) calculated with a 41% roughness.

### 3 Optical properties upon annealing

**Figure S5** shows the reflectance at normal incidence as function of the annealing temperature of the three studied systems with a 40 nm bilayer thickness. The samples were isochronically annealed at 200 °C, every 25 °C from 250 °C and 350 °C, 400 °C and again every every 25 °C from 500 °C to 600 °C. The color maps illustrate that the transition from the hyperbolic behaviour to higher reflectivities happens in the range of 300 °C to 325 °C for all three samples.

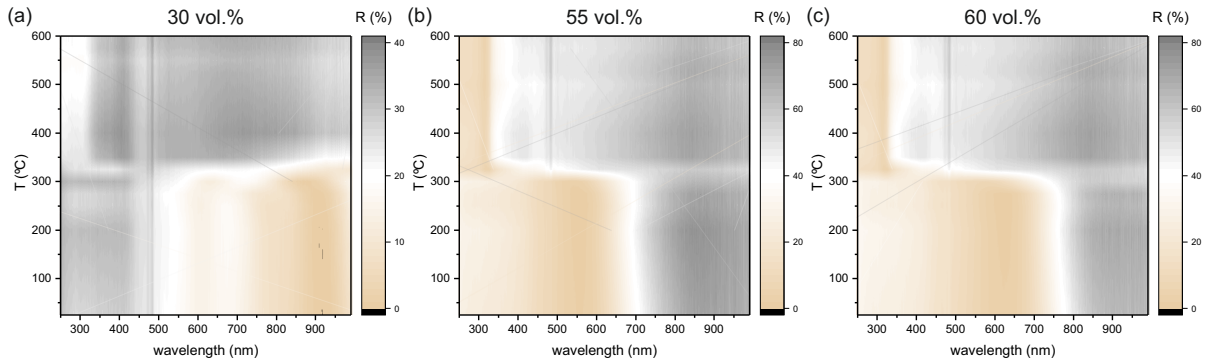

Figure S5: Evolution of the reflectivity at normal incidence of the 30 vol.% Ag system (a), 55 vol.% Ag system (b) and 60 vol.% Ag system (c) against annealing temperature.

**Figure S6** illustrates the  $R_p/R_s$  ratio in the as-deposited and annealed at 300 °C and 500 °C state of samples with different Ag content and stacking orders. The color maps of the samples with an AB stacking order show how the features related to the optical hyperbolic regime persist at 300 °C, but disappear at 500 °C. Analogous to the main text (Figure 1f) but now for systems with different bilayer thickness, the system with 30 vol.% Ag demonstrates the discontinuity in the Brewster angle and the system with 50 vol.% Ag exhibits a transition towards isotropic reflectance at 700 nm. In the case of the samples with a BA architecture (silver on top, see Figure 4), the system also undergoes a transition with the wide-angle band at 550 nm vanishing upon annealing to 500 °C. In contrast, the minima in the  $R_p/R_s$  ratio at high wavelength and angle  $\Omega$  present in all the samples annealed at 500 °C (Figure S6g,h,l) corresponds to the Brewster angle of silver.

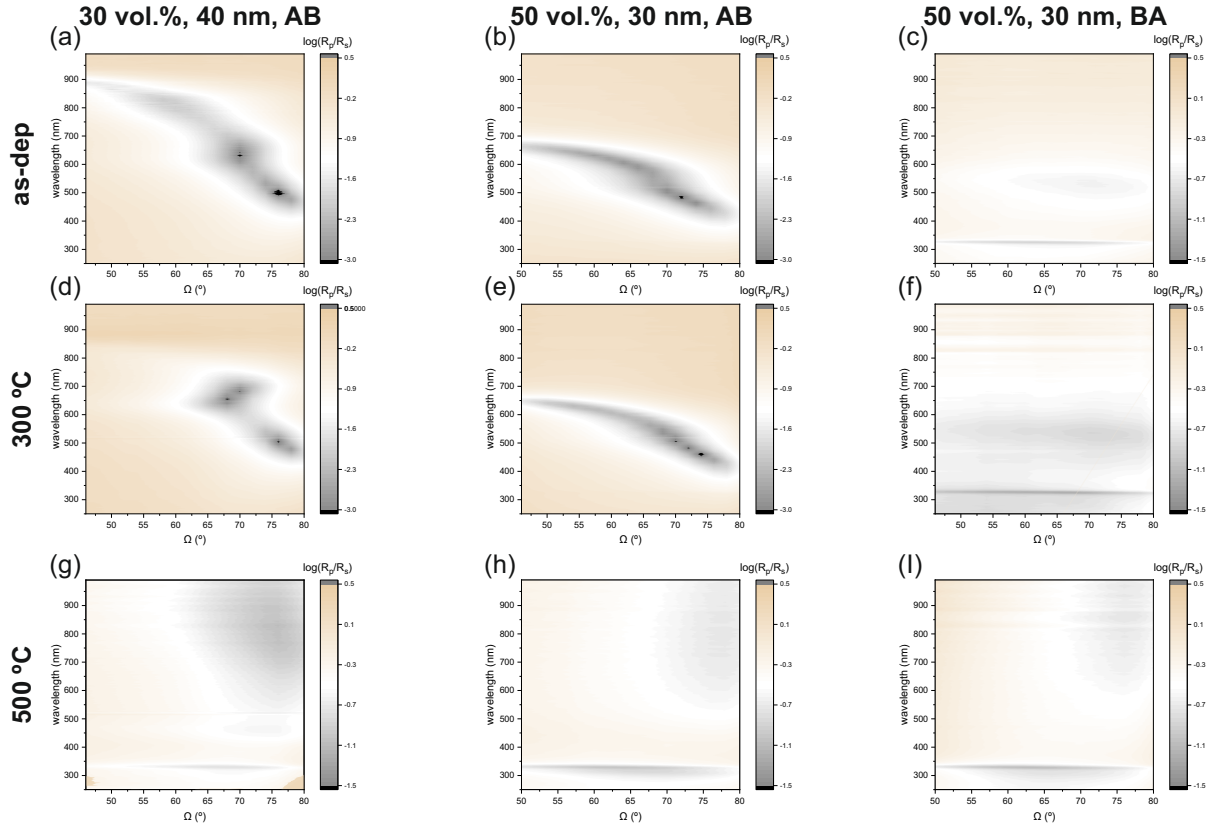

Figure S6: (a), (d) and (g): Ratio between the reflectance of p- and s-polarized light for the 30 vol.% Ag, 40 nm bilayer thickness system with AB stacking order (silicon on top) when as deposited (a) and being annealed at 300 °C (d) and 500 °C (g). (b), (e) and (h): Ratio between the reflectance of p- and s-polarized light for the 50 vol.% Ag, 30 nm bilayer thickness system with AB stacking order after deposition (b) and being annealed at 300 °C (e) and 500 °C (h). (c), (f) and (I): Ratio between the reflectance of p- and s-polarized light for of the 50 vol.% Ag, 30 nm bilayer thickness system with BA stacking order (silver on top) when as-deposited (c) and being annealed at 300 °C (f) and 500 °C (I).

## 4 Finite Element modelling

**Figure S7** illustrates how in this work FIB-nanotomography and FIB cross-sectional images were used for Finite Element Simulations. Three dimensional data sets are created by registration and classification using a trainable *Weka* segmentation algorithm [7]. The classified 2D or 3D data are import into Comsol Multiphysics 5.6 and used for full wave simulations (2D data) and solid mechanic simulations (3D data). In case of the 2D full wave simulations up to 10 data sets are used and averaged.

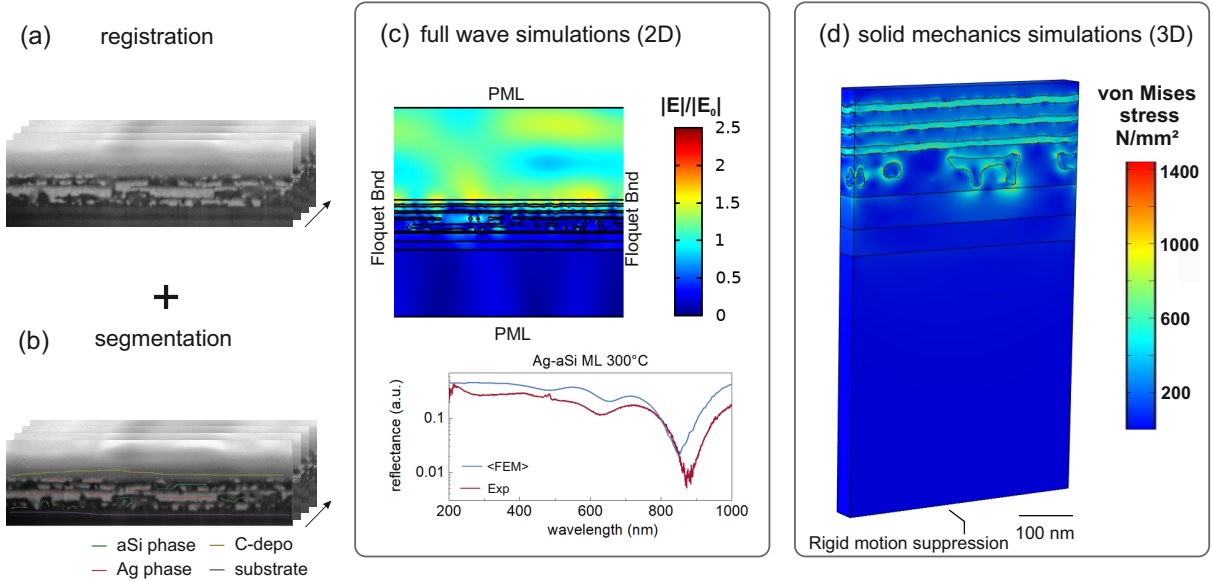

Figure S7: (a) and (b): Stacked FIB-milled cross-sections showing the process of registration (a) and segmentation (b). (c) Example of the results of a two-dimensional full wave simulation using *Comsol* and taking one of the segmented geometries shown in (b). On top, a color map of the electric field together with annotations indicating what kind of boundary conditions were used: Perfect Matched Layers (PML) and Floquet periodic boundary conditions. Below the color map, and example of the calculated reflectance compared with the experimental results. (d) Example of the results of the three-dimensional solid mechanics simulations taking a tomography build in (a) and (b) as a geometry.

## 5 Calculation of Interfacial Energy (Ag/a-Si)

**Figure S8a** shows the solubility data of Ag in a-Si as measured in Ref. [8]. The blue line is the fit used to calculate a Ag/a-Si interfacial energy of  $0.19 \text{ J/m}^2$ . This value obtained by Eq. (9) in Ref. [9] is in good agreement with calculations in literature ( $0.17 \text{ J/m}^2$ ) [10]. **Figure S8b** shows that the diffusion length of Ag in a-Si after 1 h of annealing exceeds the thickness of our multilayers at temperatures higher than  $425 \text{ }^\circ\text{C}$ , which explains the dynamics observed in **Figure 3**.

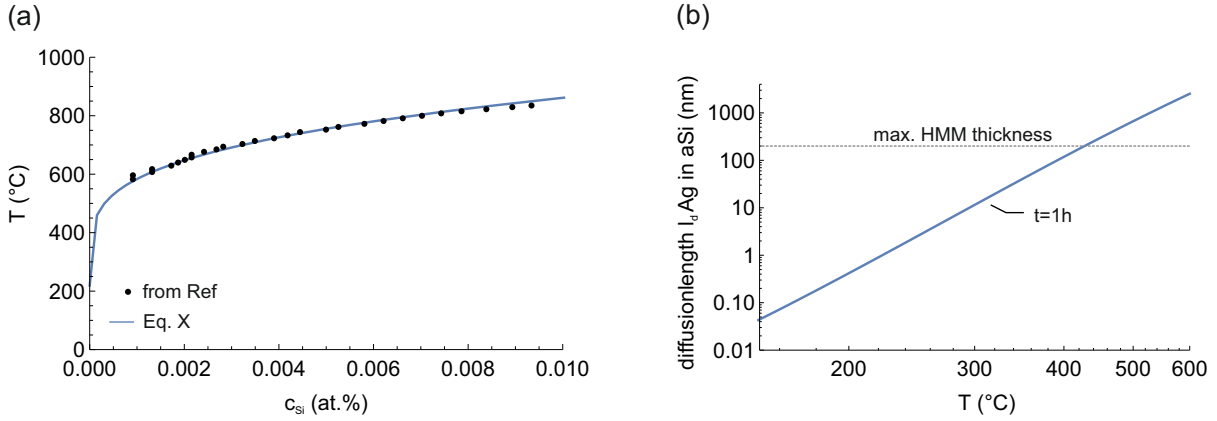

Figure S8: (a) Calculation to obtain the interfacial energy shown in the main text. (b) Plot of the diffusion length of Ag in a-Si at different temperatures using mobility data from Ref. [8].

## References

- [1] P. B. Johnson, R. W. Christy, *Phys. Rev. B* **1972**, 6 4370.
- [2] D. T. Pierce, W. E. Spicer, *Phys. Rev. B* **1972**, 5 3017.
- [3] P. Markoš, C. Soukoulis, *Wave Propagation. From Electrons to Photonic Crystals and Left-Handed Materials*, Princeton University Press, **2008**.
- [4] D. Cozza, C. M. Ruiz, D. Duché, S. Giraldo, E. Saucedo, J. J. Simon, L. Escoubas, *Opt. Express* **2016**, 24 A1201.
- [5] J. Szczyrbowski, *J. Phys. D: Appl. Phys.* **1978**, 11 583.
- [6] C. Hom-on, M. Horprathum, P. Eiamchai, S. Limwichean, V. Patthanasettakul, N. Nuntawong, C. Chananonnawathorn, T. Lertvanithphol, N. Triroj, P. Jaroenapibal, *Mater. Today: Proc.* **2018**, 5 15228.
- [7] I. Arganda-Carreras, V. Kaynig, C. Rueden, K. W. Eliceiri, J. Schindelin, A. Cardona, H. Sebastian Seung, *Bioinformatics* **2017**, 33 2424.
- [8] L. Weber, *Metall. Mater. Trans. A* **2002**, 33 1145.
- [9] P. Stender, C. B. Ene, H. Galinski, G. Schmitz, *Int. J. Mater. Res.* **2008**, 99 480.
- [10] Z. M. Wang, J. Y. Wang, L. P. H. Jeurgens, E. J. Mittemeijer, *Phys. Rev. B* **2008**, 77 045424.
